# Supplementary material for: Object as Query: Lifting any 2D Object Detector to 3D Detection
Source: arXiv:2301.02364 source file (2023-11-06)
Supplement: Supplementary file 1 [file decoder_layers.tex]

\begin{tabular}{c | c c c c c c }
\toprule[1.pt]
Layers & 1 & 2 & 3 & 4 & 5 & 6\\

\midrule
mAP & 36.4 &39.1 & 40.3 & 41.1 & 41.3 & 41.4\\ 
NDS & 44.8 & 48.7& 49.8 & 50.7 & 51.0 & 51.1\\
\bottomrule[1.pt]
\end{tabular}
